# Supplementary material for: EvIcon: Designing High-Usability Icon with Human-in-the-loop Exploration and IconCLIP
Source: arXiv:2305.17609 source file (2023-05-28)
Supplement: Supplementary file 1 [file appendix.tex]

\input{supp_data_collection}
